# Supplementary material for: Fully Tunable Strong Spin-Orbit Interactions in Light Hole Germanium Quantum Channels
Source: arXiv:2506.14759 ancillary file (2025-06-17)
Supplement: Supplementary file 1 [file si.pdf]

# Fully Tunable Strong Spin-Orbit Interactions in Light Hole Germanium Quantum Channels

Patrick Del Vecchio,[1,2,*] Stefano Bosco,[2] Daniel Loss,[3] and Oussama Moutanabbir[1,†]

[1]*Department of Engineering Physics, École Polytechnique de Montréal, Montréal, C.P. 6079, Succ. Centre-Ville, Montréal, Québec, Canada H3C 3A7*

[2]*QuTech and Kavli Institute of Nanoscience, Delft University of Technology, Delft, Netherlands*

[3]*Department of Physics, University of Basel, Klingelbergstrasse 82, 4056 Basel, Switzerland*

**Appendix A: 6-band $k\cdot p$ theoretical framework**

6-band $k\cdot p$ theory is employed to evaluate the energy and probability densities of the planar heterostructure subbands. Each subband $j$ with pseudo-spin $\sigma=\pm1$ is associated with a 3-component spinor with envelope function components $f_j^{\nu}(z)\equiv\langle z|f_j^{\nu}\rangle$, where $\nu=\{\ell,s,h\}$ refer to LH, split-off hole and HH bands, respectively. For quantum wells grown on [001]-oriented substrates, and with $k_x=k_y=0$ and $B=0$, the eigenstates of the system are solutions of the following subband-edge Hamiltonian [1, 2]:

$$H_0^{\mathrm{QW}}=\begin{bmatrix}H_{\sigma=+} & 0\\ 0 & H_{\sigma=-}\end{bmatrix}, \tag{A1a}$$

$$H_\sigma=H_\sigma^k+H_\sigma^\varepsilon+V, \tag{A1b}$$

where

$$H_\sigma^k=\alpha_0\begin{bmatrix}-k_z\gamma_+k_z & 2\sqrt{2}\sigma k_z\gamma_2k_z & 0\\ & -k_z\gamma_1k_z & 0\\ \dagger & & -k_z\gamma_-k_z\end{bmatrix}, \tag{A2a}$$

$$H_\sigma^\varepsilon=a_v\mathrm{Tr}\,\varepsilon+b\cdot\delta\varepsilon\begin{bmatrix}-1 & \sqrt{2}\sigma & 0\\ & 0 & 0\\ \dagger & & 1\end{bmatrix}, \tag{A2b}$$

$$V=\mathcal{E}_{\Gamma_5^+}+\frac{\Delta_0}{3}+eF_zz-\Delta_0\begin{bmatrix}0&0&0\\ &1&0\\ \dagger & & 0\end{bmatrix}, \tag{A2c}$$

where $\gamma_\pm=\gamma_1\pm2\gamma_2$ are Luttinger parameters, $a_v$ and $b$ are strain deformation potentials, $\delta\varepsilon=\varepsilon_{xx}-\varepsilon_{zz}$, where $\varepsilon_{ij}$ is the strain tensor, $\Delta_0$ is the bulk split-off gap, and $\mathcal{E}_{\Gamma_5^+}$ is the valence band edge energy without spin-orbit coupling.

It can be seen from (A1a) that only the component $\nu=h$ contributes to a HH subband, while LH levels get contributions from one dominant $\nu=\ell$ spinor component and one weaker $\nu=s$ component. More explicitly,

$$|\mathrm{H}\sigma;l\rangle=\left|\frac{3}{2},\frac{3\sigma}{2}\right\rangle\left|f_l^h\right\rangle, \tag{A3a}$$

$$|\mathrm{L}\sigma;j\rangle=\left|\frac{3}{2},\frac{\sigma}{2}\right\rangle\left|f_j^\ell\right\rangle+\sigma\left|\frac{1}{2},\frac{\sigma}{2}\right\rangle\left|f_j^s\right\rangle, \tag{A3b}$$

where the shorthands "H" and "L" refer to HH and LH subbands, respectively, and where the $|J,M_J\rangle$ are bulk Bloch states. At $k_x=k_y=0$ and $B=0$, $|\mathrm{L}\sigma;j\rangle$ and $|\mathrm{H}\sigma;l\rangle$ have $\sigma$-independent energies $E_j^{\mathrm{L}}$ and $E_l^{\mathrm{H}}$ respectively.

Each material parameter ($\gamma_1$, $a_v$, $\mathcal{E}_{\Gamma_5^+}$, …) is a function of $z$, which in the Hamiltonian (A1a) translates to diagonal operators in position basis $|z\rangle$, i.e.


* p.delvecchio@tudelft.nl

† oussama.moutanabbir@polymtl.ca

$$\gamma_1 \left| z \right\rangle = \left| z \right\rangle \gamma_1(z), \tag{A4}$$

where $\gamma_1$ is an *operator* and $\gamma_1(z)$ is a function returning the value of $\gamma_1$ at position $z$ (and similarly with all other parameters). This implies that the operator ordering must be exactly as it is shown in (A1a), since in general, material operators do not commute with $k_z$. Since eigenstates of $H_+$ are degenerate with those of $H_-$, it suffices to diagonalize only $H_+$, and then construct the eigenstates of $H_-$ from time-reversal rules.

Away from $k_x = k_y = 0$ and with $\mathbf{B} = B\mathbf{e}_z$, the eigenstates of (A1a) provide an orthonormal basis on which the full $k \cdot p$ Hamiltonian can be projected. This gives (with bold characters indicating matrices expressed in the eigenbasis of $H_0^{\mathrm{QW}}$)

$$\mathbf{H}^{\mathrm{QW}} = \mathbf{E}_0^{\mathrm{QW}} + \alpha_0 \mathbf{M}_\gamma K_\parallel^2 + \frac{\alpha_0}{2l_B^2}\mathbf{M}_g + \alpha_0 \left( i\mathbf{M}_1 K_- + \mathbf{M}_2 K_-^2 + \text{h.c.} \right), \tag{A5}$$

where $K_\pm = K_x \pm iK_y$, $K_\parallel^2 = K_x^2 + K_y^2 = \{K_-, K_+\}/2$, and

$$\mathbf{E}_0^{\mathrm{QW}} = \begin{bmatrix} \mathbf{E}^{\mathrm{H}} & 0 & 0 & 0 \\ & \mathbf{E}^{\mathrm{L}} & 0 & 0 \\ & & \mathbf{E}^{\mathrm{L}} & 0 \\ & & & \mathbf{E}^{\mathrm{H}} \end{bmatrix}, \tag{A6}$$

with $\mathbf{E}^\tau = \mathrm{diag}\{E_1^\tau, E_2^\tau, \dots\}$ ($\tau = \{\mathrm{L}, \mathrm{H}\}$) are the energies from (A1a). The $\mathbf{M}$-matrices are

$$\mathbf{M}_\gamma = \begin{bmatrix} \mathbf{\Gamma}_\parallel^{\mathrm{H}} & 0 & 0 & 0 \\ & \mathbf{\Gamma}_\parallel^{\mathrm{L}} & 0 & 0 \\ & & \mathbf{\Gamma}_\parallel^{\mathrm{L}} & 0 \\ & & & \mathbf{\Gamma}_\parallel^{\mathrm{H}} \end{bmatrix}, \qquad \mathbf{M}_g = \begin{bmatrix} \mathbf{G}_\perp^{\mathrm{H}} & 0 & 0 & 0 \\ & \mathbf{G}_\perp^{\mathrm{L}} & 0 & 0 \\ & & -\mathbf{G}_\perp^{\mathrm{L}} & 0 \\ & & & -\mathbf{G}_\perp^{\mathrm{H}} \end{bmatrix}, \tag{A7a}$$

$$\mathbf{M}_1 = \begin{bmatrix} 0 & \mathbf{T}^{\mathrm{x}} & 0 & 0 \\ 0 & 0 & \mathbf{T}^{\mathrm{L}} & 0 \\ 0 & 0 & 0 & \mathbf{T}^{\mathrm{x}\dagger} \\ \mathbf{T}^{\mathrm{H}} & 0 & 0 & 0 \end{bmatrix}, \qquad \mathbf{M}_2 = \begin{bmatrix} 0 & 0 & \boldsymbol{\mu} & 0 \\ 0 & 0 & 0 & \boldsymbol{\mu}^\dagger \\ \boldsymbol{\delta}^\dagger & 0 & 0 & 0 \\ 0 & \boldsymbol{\delta} & 0 & 0 \end{bmatrix}. \tag{A7b}$$

Matrix elements within $\mathbf{M}$-matrices are further expanded in terms of the eigenstates of (A1a):

$$\mathbf{\Gamma}_{\parallel}^{\mathrm{H}} = -\langle f^h|\gamma_1 + \gamma_2|f^h\rangle\,, \tag{A8a}$$

$$\mathbf{G}_{\perp}^{\mathrm{H}} = -\langle f^h|6\kappa + \frac{27q}{2}|f^h\rangle\,, \tag{A8b}$$

$$\mathbf{\Gamma}_{\parallel}^{\mathrm{L}} = -\langle f^z|\gamma_-|f^z\rangle - \langle f^\circ|\gamma_1 + \gamma_2|f^\circ\rangle\,, \tag{A8c}$$

$$\mathbf{G}_{\perp}^{\mathrm{L}} = -6\,\langle f^\circ|\kappa|f^\circ\rangle - \frac{1}{2}\,\langle f^\ell|q|f^\ell\rangle + 2\left(\langle f^z|f^z\rangle - 2\,\langle f^\circ|f^\circ\rangle\right), \tag{A8d}$$

$$\mathbf{T}^{\mathrm{x}} = -\frac{3i}{\sqrt{2}}\,\langle f^h|\left(u_+\,|f^z\rangle + \frac{7\sqrt{6}}{12}[q,k_z]\,|f^\ell\rangle\right), \tag{A8e}$$

$$\mathbf{T}^{\mathrm{H}} = -\frac{3i}{2}\,\langle f^h|[q,k_z]|f^h\rangle\,, \tag{A8f}$$

$$\mathbf{T}^{\mathrm{L}} = -\frac{3i}{\sqrt{2}}\left(\langle f^\circ|u_+|f^z\rangle - \langle f^z|u_-|f^\circ\rangle\right) - 5i\,\langle f^\ell|[q,k_z]|f^\ell\rangle\,, \tag{A8g}$$

$$\boldsymbol{\mu} = \frac{3}{2}\,\langle f^h|\gamma_2 + \gamma_3|f^\circ\rangle\,, \tag{A8h}$$

$$\boldsymbol{\delta} = \frac{3}{2}\,\langle f^h|\gamma_2 - \gamma_3|f^\circ\rangle\,, \tag{A8i}$$

where $u_\pm = \{\gamma_3, k_z\} \pm [\kappa, k_z]$, $\{A,B\} \equiv AB + BA$ is the anti-commutator and

$$|f_j^z\rangle \equiv \frac{1}{\sqrt{3}}\left(\sqrt{2}\,|f_j^\ell\rangle - |f_j^s\rangle\right), \tag{A9a}$$

$$|f_j^\circ\rangle \equiv \frac{1}{\sqrt{3}}\left(|f_j^\ell\rangle + \sqrt{2}\,|f_j^s\rangle\right). \tag{A9b}$$

Subband indices have been omitted for simplicity.

The quantum channel Hamiltonian eigenstates $|\tilde{\sigma}; i, N\rangle$ with associated energy $E^c_{i,N}$ at $k_y = 0$ and $B = 0$ are calculated from (A5) by setting $k_y = 0$ and by introducing a parabolic confinement potential $-\alpha_0 x^2/l_x^4$:

$$\mathbf{H}_0^{\mathrm{QC}} = \mathbf{E}_0^{\mathrm{QW}} + \alpha_0 \mathbf{M}_\gamma k_x^2 + \alpha_0\left(i\mathbf{M}_1 k_x + \mathbf{M}_2 k_x^2 + \mathrm{h.c.}\right) - \frac{\alpha_0}{l_x^4}x^2. \tag{A10}$$

Projecting this Hamiltonian onto an in-plane basis of harmonic oscillator eigenstates $|n\rangle$ (with $a^\dagger a\,|n\rangle = |n\rangle\,n$, $a\,|n\rangle = |n-1\rangle\sqrt{n}$ and $a^\dagger\,|n\rangle = |n+1\rangle\sqrt{n+1}$), with

$$a = \frac{1}{\sqrt{2}}\left(\frac{x}{l_x} + i l_x k_x\right), \tag{A11}$$

provides and eigenbasis of quantum channel subband edges on which the full quantum channel Hamiltonian away from $k_y = 0$ and $B = 0$ is projected. The result is

$$\mathbf{H}^{\mathrm{QC}} = \mathbf{E}_0^{\mathrm{QC}} + \alpha_0\left(\mathbf{L}_1 k_y + \mathbf{L}_\gamma k_y^2 + \frac{1}{2l_B^2}\mathbf{L}_g + \frac{1}{2l_B^2}\mathbf{L}_3 k_y + \frac{1}{4l_B^4}\mathbf{L}_4\right), \tag{A12}$$

where

$$\mathbf{E}_0^{\text{QC}} = \begin{bmatrix} \mathbf{E}^c & 0 \\ 0 & \mathbf{E}^c \end{bmatrix}, \tag{A13}$$

and $\mathbf{E}^c = \text{diag}\{E^c_{1,0}, E^c_{1,1}, \ldots, E^c_{2,0}, E^c_{2,1}, \ldots\}$. Some $\mathbf{L}$-matrices are further expanded into $\theta$-independent $\mathbf{L}$-matrices:

$$\mathbf{L}_g = \mathbf{L}_{g\perp}\cos\theta + \mathbf{L}_{g\|}\sin\theta, \tag{A14a}$$
$$\mathbf{L}_3 = \mathbf{L}_{3\perp}\cos\theta + \mathbf{L}_{3\|}\sin\theta, \tag{A14b}$$
$$\mathbf{L}_4 = \mathbf{L}_{4\perp}\cos^2\theta + \mathbf{L}_{4\|}\sin^2\theta + \mathbf{L}_{4\times}\sin\theta\cos\theta. \tag{A14c}$$

Just like the $\mathbf{M}$-matrices in the QW Hamiltonian, the $\mathbf{L}$-matrices in the QC system are computed from the eigenstates of the QC Hamiltonian at $k_y = 0$ and $B = 0$:

$$\mathbf{L}_1 = \mathbf{T}^c\tilde{\sigma}_1 = \langle\tilde{\sigma}; i, N|\, \mathbf{m}_1 - 2\mathbf{m}_2 k_x \,|\tilde{\sigma}'; i', N'\rangle, \tag{A15a}$$
$$\mathbf{L}_\gamma = \mathbf{\Gamma}^c\tilde{\sigma}_0 = \langle\tilde{\sigma}; i, N|\, \mathbf{m}_0 \,|\tilde{\sigma}'; i', N'\rangle, \tag{A15b}$$
$$\mathbf{L}_{g\perp} = \mathbf{G}^c_\perp\tilde{\sigma}_3 = \langle\tilde{\sigma}; i, N|\, \mathbf{M}_g + 2\mathbf{m}_1 x - 2\mathbf{m}_2\{x, k_x\} \,|\tilde{\sigma}'; i', N'\rangle, \tag{A15c}$$
$$\mathbf{L}_{g\|} = \mathbf{G}^c_\|\tilde{\sigma}_2 = \langle\tilde{\sigma}; i, N|\, \mathbf{n}_g - \mathbf{N}'_\gamma x + \mathbf{n}'_1\{x, k_x\} \,|\tilde{\sigma}'; i', N'\rangle, \tag{A15d}$$
$$\mathbf{L}_{3\perp} = \mathbf{\Xi}_\perp\tilde{\sigma}_2 = 4\,\langle\tilde{\sigma}; i, N|\, \mathbf{m}_0 x \,|\tilde{\sigma}'; i', N'\rangle, \tag{A15e}$$
$$\mathbf{L}_{3\|} = \mathbf{\Xi}_\|\tilde{\sigma}_3 = 2\,\langle\tilde{\sigma}; i, N|\, \mathbf{n}_1 x \,|\tilde{\sigma}'; i', N'\rangle, \tag{A15f}$$
$$\mathbf{L}_{4\perp} = \mathbf{Z}_\perp\tilde{\sigma}_0 = 4\,\langle\tilde{\sigma}; i, N|\, \mathbf{m}_0 x^2 \,|\tilde{\sigma}'; i', N'\rangle, \tag{A15g}$$
$$\mathbf{L}_{4\|} = \mathbf{Z}_\|\tilde{\sigma}_0 = \langle\tilde{\sigma}; i, N|\, \mathbf{N}_\gamma x^2 \,|\tilde{\sigma}'; i', N'\rangle, \tag{A15h}$$
$$\mathbf{L}_{4\times} = \mathbf{Z}_\times\tilde{\sigma}_1 = 4\,\langle\tilde{\sigma}; i, N|\, \mathbf{n}_1 x^2 \,|\tilde{\sigma}'; i', N'\rangle, \tag{A15i}$$

with $\tilde{\sigma}_0$ the $2\times 2$ identity matrix and $\tilde{\sigma}_{1,2,3}$ the Pauli matrices. The $\mathbf{m}$ and $\mathbf{n}$ matrices are

$$\mathbf{m}_0 = \mathbf{M}_\gamma - \mathbf{M}_2 - \mathbf{M}_2^\dagger, \tag{A16a}$$
$$\mathbf{m}_1 = \mathbf{M}_1 + \mathbf{M}_1^\dagger, \tag{A16b}$$
$$\mathbf{m}_2 = i(\mathbf{M}_2 - \mathbf{M}_2^\dagger), \tag{A16c}$$
$$\mathbf{n}_g = -i(\mathbf{N}_g - \mathbf{N}_g^\dagger), \tag{A16d}$$
$$\mathbf{n}_1 = \mathbf{N}_1 + \mathbf{N}_1^\dagger, \tag{A16e}$$
$$\mathbf{n}'_1 = i(\mathbf{N}_1 - \mathbf{N}_1^\dagger). \tag{A16f}$$

with

$$\mathbf{N}_\gamma = 4\begin{bmatrix} \mathbf{\Gamma}^{\text{H}}_\perp & 0 & 0 & 0 \\ 0 & \mathbf{\Gamma}^{\text{L}}_\perp & 0 & 0 \\ 0 & 0 & \mathbf{\Gamma}^{\text{L}}_\perp & 0 \\ 0 & 0 & 0 & \mathbf{\Gamma}^{\text{H}}_\perp \end{bmatrix}, \qquad \mathbf{N}'_\gamma = 4\begin{bmatrix} \mathbf{\Gamma}'^{\text{H}}_\perp & 0 & 0 & 0 \\ 0 & \mathbf{\Gamma}'^{\text{L}}_\perp & 0 & 0 \\ 0 & 0 & \mathbf{\Gamma}'^{\text{L}}_\perp & 0 \\ 0 & 0 & 0 & \mathbf{\Gamma}'^{\text{H}}_\perp \end{bmatrix}, \tag{A17}$$

$$\mathbf{N}_g = \begin{bmatrix} 0 & \mathbf{G}^{\text{x}}_\| & 0 & 0 \\ 0 & 0 & \mathbf{G}^{\text{L}}_\| & 0 \\ 0 & 0 & 0 & \mathbf{G}^{\text{x}\dagger}_\| \\ \mathbf{G}^{\text{H}}_\| & 0 & 0 & 0 \end{bmatrix}, \qquad \mathbf{N}_1 = \begin{bmatrix} 0 & \mathbf{R}^{\text{x}}_\| & 0 & 0 \\ 0 & 0 & \mathbf{R}^{\text{L}}_\| & 0 \\ 0 & 0 & 0 & \mathbf{R}^{\text{x}\dagger}_\| \\ 0 & 0 & 0 & 0 \end{bmatrix}, \tag{A18}$$

where

$$\mathbf{\Gamma}^{\rm L} = -\langle f^\circ|\gamma_-|f^\circ\rangle - \langle f^z|\gamma_1+4\gamma_2|f^z\rangle\,, \tag{A19a}$$

$$\mathbf{\Gamma}^{\rm H} = -\langle f^h|\gamma_-|f^h\rangle\,, \tag{A19b}$$

$$\mathbf{\Gamma}'^{\rm L} = -\frac{1}{2}\left(\langle f^\circ|\{\gamma_-,k_z\}|f^\circ\rangle + \langle f^z|\{\gamma_1+4\gamma_2,k_z\}|f^z\rangle\right), \tag{A19c}$$

$$\mathbf{\Gamma}'^{\rm H} = -\frac{1}{2}\langle f^h|\{\gamma_-,k_z\}|f^h\rangle\,, \tag{A19d}$$

$$\mathbf{G}_\parallel^{\rm x} = -\sqrt{2}\,\langle f^h|\left(3\kappa\,|f^z\rangle + \frac{7\sqrt{6}q}{4}\,|f^\ell\rangle - \sqrt{3}\,|f^s\rangle\right), \tag{A19e}$$

$$\mathbf{G}_\parallel^{\rm L} = -\sqrt{2}\,\langle f^\circ|3\kappa+1|f^z\rangle - \sqrt{2}\,\langle f^z|3\kappa+1|f^\circ\rangle + 2\,\langle f^z|f^z\rangle - 10\,\langle f^\ell|q|f^\ell\rangle\,, \tag{A19f}$$

$$\mathbf{G}_\parallel^{\rm H} = -3\,\langle f^h|q|f^h\rangle\,, \tag{A19g}$$

$$\mathbf{R}^{\rm x} = 3\sqrt{2}i\,\langle f^h|\gamma_3|f^z\rangle\,, \tag{A19h}$$

$$\mathbf{R}^{\rm L} = 3\sqrt{2}i\left(\langle f^\circ|\gamma_3|f^z\rangle - \langle f^z|\gamma_3|f^\circ\rangle\right). \tag{A19i}$$

The quantum dot system eigenstates $|\tilde{\sigma};i,N_1,N_2\rangle$, with associated energy $E^d_{i,N_1,N_2}$, are calculated at $B=0$ similarly to those of the QC system, i.e., by introducing into (A5) an in-plane parabolic potential $-\alpha_0\left(x^2/l_x^4+y^2/l_y^4\right)$:

$$\mathbf{H}_0^{\rm QD} = \mathbf{E}_0^{\rm QW} + \alpha_0\left[\mathbf{M}_\gamma k_\parallel^2 + \left(i\mathbf{M}_1k_- + \mathbf{M}_2k_-^2 + \text{h.c.}\right)\right] - \alpha_0\left(\frac{x^2}{l_x^4}+\frac{y^2}{l_y^4}\right), \tag{A20}$$

and by projecting the in-plane degrees of freedom onto a harmonic oscillator basis, acted upon by the following two ladder operators:

$$a_1 = \frac{1}{\sqrt{2}}\left(\frac{x}{l_x}+il_xk_x\right), \qquad a_2 = \frac{1}{\sqrt{2}}\left(\frac{y}{l_y}+il_yk_y\right). \tag{A21}$$

The $a_i$'s satisfy $[a_i,a_j^\dagger]=\delta_{i,j}$. Eigenstates of (A20) provide an orthonormal basis on which the full $k\cdot p$ Hamiltonian with $B>0$ can be projected. The result is (with $B$ lying in the $y$-$z$ plane)

$$\begin{aligned}\mathbf{H}^{\rm QD} = \mathbf{E}_0^{\rm QD} + \frac{\alpha_0}{2l_B^2}\Bigg\{&\cos\theta\mathbf{L}_{2\perp} + \frac{\cos^2\theta}{2l_B^2}\mathbf{L}_{4\perp} + \frac{\sin^2\theta}{2l_B^2}\mathbf{L}_{4\parallel}\\ &-\sin\theta\left[i\mathbf{L}_{2\parallel} + \frac{\sin\theta}{2l_B^2}\mathbf{L}'_{4\parallel} + i\frac{\cos\theta}{2l_B^2}\mathbf{L}_{4\times} + \text{h.c.}\right]\Bigg\},\end{aligned} \tag{A22}$$

where

$$\mathbf{E}_0^{\rm QD} = \begin{bmatrix}\mathbf{E}^d & 0\\ 0 & \mathbf{E}^d\end{bmatrix} \tag{A23}$$

with $\mathbf{E}^d = \text{diag}\{E^d_{1,0,0},E^d_{1,0,1},\dots\}$ are the eigenvalues of (A20) and the $\mathbf{L}$-matrices are expanded in terms of the eigenstates of (A20):

$$
\begin{aligned}
\mathbf{L}_{2\perp} &= \mathbf{G}_{\perp}^{d}\tilde{\sigma}_{+}\tilde{\sigma}_{-} + \mathbf{G}_{\perp}^{d*}\tilde{\sigma}_{-}\tilde{\sigma}_{+} && \text{(A24a)}\\
&= \langle\tilde{\sigma}; i, N_1, N_2|\, \mathbf{M}_g + [i\mathbf{M}_\gamma\{\zeta_+, k_-\} + 2\mathbf{M}_1\zeta_- - 4i\mathbf{M}_2\zeta_- k_- + \text{h.c.}]\, |\tilde{\sigma}'; i', N_1', N_2'\rangle\,, \\
\mathbf{L}_{2\parallel} &= \mathbf{G}_{+}^{d}\tilde{\sigma}_{+} + \mathbf{G}_{-}^{d}\tilde{\sigma}_{-} && \text{(A24b)}\\
&= \langle\tilde{\sigma}; i, N_1, N_2|\, \mathbf{N}_g - i\mathbf{N}_\gamma'\zeta_+ - \mathbf{N}_1\{\zeta_+, k_-\} + 2\mathbf{N}_1^\dagger\zeta_+ k_+\, |\tilde{\sigma}'; i', N_1', N_2'\rangle\,, \\
\mathbf{L}_{4\perp} &= \langle\tilde{\sigma}; i, N_1, N_2|\, 4\mathbf{M}_\gamma\zeta_+\zeta_- - 4\left[\mathbf{M}_2\zeta_-^2 + \text{h.c.}\right] |\tilde{\sigma}'; i', N_1', N_2'\rangle && \text{(A24c)}\\
\mathbf{L}_{4\parallel} &= \langle\tilde{\sigma}; i, N_1, N_2|\, 2\mathbf{N}_\gamma\zeta_+\zeta_-\, |\tilde{\sigma}'; i', N_1', N_2'\rangle && \text{(A24d)}\\
\mathbf{L}_{4\parallel}' &= -\langle\tilde{\sigma}; i, N_1, N_2|\, \mathbf{N}_\gamma\zeta_+^2\, |\tilde{\sigma}'; i', N_1', N_2'\rangle && \text{(A24e)}\\
\mathbf{L}_{4\times} &= 4i\,\langle\tilde{\sigma}; i, N_1, N_2|\, \mathbf{N}_1\zeta_+\zeta_- + \mathbf{N}_1^\dagger\zeta_+^2\, |\tilde{\sigma}'; i', N_1', N_2'\rangle && \text{(A24f)}
\end{aligned}
$$

with $\tilde{\sigma}_\pm = (\tilde{\sigma}_1 \pm i\tilde{\sigma}_2)/2$ and $\zeta_\pm = (x \pm iy)/2$. The ground state two-level system with energy $\hbar\omega$ is computed by diagonalizing (A22) with $B = 0.05\,\text{T}$.

The fan-diagram calculations of section E below are performed by diagonalizing (A5) in the axial approximation (which corresponds to $\boldsymbol{\delta} = 0$ in $\mathbf{M}_2$), and by writing $K_-$ in terms of the ladder operator

$$
a = \frac{i l_B K_-}{\sqrt{2}}. \qquad \text{(A25)}
$$

Inserting this into (A5) reveals that all eigenstates must be of the form

$$
|\varphi\rangle = \begin{bmatrix} |m-1\rangle\, \mathbf{c}_{\mathrm{H}+} \\ |m\rangle\, \mathbf{c}_{\mathrm{L}+} \\ |m+1\rangle\, \mathbf{c}_{\mathrm{L}-} \\ |m+2\rangle\, \mathbf{c}_{\mathrm{H}-} \end{bmatrix}, \qquad \text{(A26)}
$$

where $m$ is an integer labeling Landau levels and $\mathbf{c}_{\tau\sigma}$ are vectors of coefficients. Following the approach outlined in Reference 3, replacing all the $a$'s within the Hamiltonian by the corresponding $m$, the fan-diagram is readily computed for as many Landau levels $m \geq -2$ as required.

#### Appendix B: Perturbative framework

Perturbative expansions of the effective parameters in the quantum well and quantum channel systems are obtained by means of a Schrieffer-Wolff transformation (SWT). The subspace for which the effective Hamiltonian is constructed is two dimensional, and consists of the ground state subband with pseudo-spin $\sigma$, or $\tilde{\sigma}$ for QWs and QCs, respectively. Remote bands consist of all other subbands. Taking (A5) or (A12), the part with known eigenvalues are the $\mathbf{E}_0$ matrices, while the perturbation is the remaining terms.

The linear Rashba parameter $\beta_1^p$ of the QW ground state L1 is exactly described by a first order SWT. It is given by

$$\beta_1^p = \alpha_0 T_{1,1}^{\mathrm{L}}, \tag{B1}$$

where $T_{1,1}^{\mathrm{L}}$ belongs to the $\mathbf{M}_1$ matrix described in Section A. The $g$-factor component $g_\perp^p$ is given exactly by a 2$^{\mathrm{nd}}$ order SWT. It is given by

$$g_\perp^p = G_{\perp;1,1}^{\mathrm{L}} + 2\alpha_0 \left[ \sum_{j\neq 1} \frac{T_{1,j}^{\mathrm{L}} T_{j,1}^{\mathrm{L}}}{E_1^{\mathrm{L}} - E_j^{\mathrm{L}}} - \sum_l \frac{\left(T_{l,1}^{\mathrm{x}}\right)^* T_{l,1}^{\mathrm{x}}}{E_1^{\mathrm{L}} - E_l^{\mathrm{H}}} \right]. \tag{B2}$$

For the QC effective parameters $g_{\perp,\parallel}^c$ and $\beta_1^c$, only a 1$^{\mathrm{st}}$ order SWT is required for an exact description. They are given directly by the corresponding matrix elements in the $\mathbf{L}$ matrices described above (with $i = 1$ and $N = 0$):

$$g_\perp^c = G_{\perp;1,0}^c \tag{B3}$$

$$g_\parallel^c = G_{\parallel;1,0}^c \tag{B4}$$

$$\beta_1^c = \alpha_0 T_{1,0}^c. \tag{B5}$$

## Appendix C: Additional ground state parameters of the QW system

Similarly to $\beta_1^p$, the other two cubic Rashba parameters $\beta_{2,3}^p$ can be evaluated as a function of $l_z$ and $F_z$. The result is shown in Fig. 1. Note that in contrast to HH systems, $\gamma_3^p > \gamma_2^p$ for LH levels.

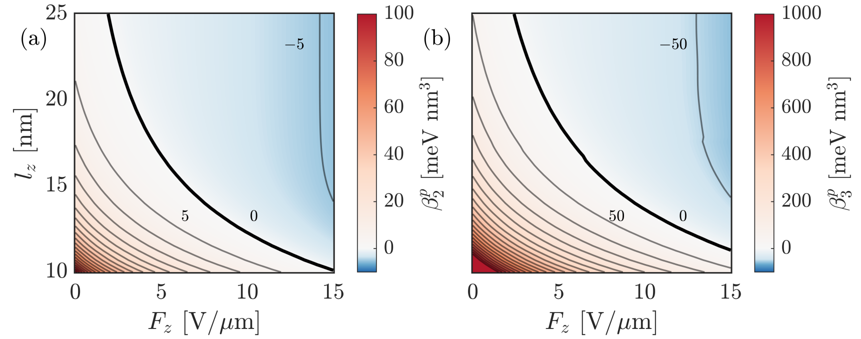


FIG. 1. Cubic Rashba parameters $\beta_2^p$ and $\beta_3^p$ as a function of $l_z$ and $F_z$, with Sn content $x = 16\%$.

### Appendix D: Derivation of the estimation for $g_\perp^c$

Starting from the effective Hamiltonian for the QW ground state L1, and only considering the effective mass term, the Zeeman splitting term, the linear Rashba term and the parabolic confinement along $x$, one gets

$$H_{\text{eff}}^p = H_0 + W, \tag{D1}$$

where

$$H_0 = \alpha_0 \gamma_\parallel^p K_\parallel^2 + \frac{\alpha_0}{2 l_B^2} g_\perp^p \sigma_z - \alpha_0 \frac{x^2}{l_x^4} \tag{D2}$$

$$W = i\beta_1^p K_- \sigma_+ + \text{h.c.} \tag{D3}$$

The part $H_0$ without linear Rashba is easily diagonalized by writing $x$ and the wavevector components in terms of ladder operators

$$a = \frac{1}{\sqrt{2}} \left( \frac{x}{\lambda_x} + i\lambda_x k_x \right), \tag{D4}$$

with $\lambda_x^4 = -\gamma_\parallel^p l_x^4$ chosen such that the Hamiltonian is readily diagonalized. With $\mathbf{B} = B\mathbf{e}_z$ and $k_y = 0$, the mechanical wavevector components become

$$K_x = k_x = \frac{1}{\sqrt{2} i \lambda_x} \left( a - a^\dagger \right) \tag{D5}$$

$$K_y = 0 + \frac{x}{l_B^2} = \frac{\lambda_x}{\sqrt{2} l_B^2} (a + a^\dagger). \tag{D6}$$

Neglecting quadratic-in-$B$ terms, the eigenvalues of $H_0$ (denoted by $E_{n\sigma}^{(0)}$) are

$$E_{n\sigma}^{(0)} = -\frac{\alpha_0 \sqrt{-\gamma_\parallel^p}}{l_x^2} (2n+1) + \frac{\alpha_0}{2 l_B^2} g_\perp^p \sigma \tag{D7}$$

with $\sigma = \pm 1$ and $n \geq 0$ being the eigenvalue of $a^\dagger a \left| n \right\rangle = \left| n \right\rangle n$. Contributions to the energy from the linear Rashba term $W$ are treated by simple perturbation theory. While 1st order perturbation gives no contributions, 2nd order perturbation gives

$$E_{0+}^{(2)} = \sum_{n'\sigma'} \frac{\left| \langle 0+ | W | n'\sigma' \rangle \right|^2}{E_{0+}^{(0)} - E_{n'\sigma'}^{(0)}} \approx \frac{(\beta_1^p l_x)^2}{4\alpha_0 \sqrt{-\gamma_\parallel^p}} \left( \frac{1}{\lambda_x^2} + \frac{2}{l_B^2} \right), \tag{D8}$$

$$E_{0-}^{(2)} = \sum_{n'\sigma'} \frac{\left| \langle 0- | W | n'\sigma' \rangle \right|^2}{E_{0-}^{(0)} - E_{n'\sigma'}^{(0)}} \approx \frac{(\beta_1^p l_x)^2}{4\alpha_0 \sqrt{-\gamma_\parallel^p}} \left( \frac{1}{\lambda_x^2} - \frac{2}{l_B^2} \right). \tag{D9}$$

Subtracting $E_{0-} = E_{0-}^{(0)} + E_{0-}^{(2)}$ from $E_{0+} = E_{0+}^{(0)} + E_{0+}^{(2)}$ gives an approximation for the Zeeman splitting energy of the QC ground state. Multiplying by $l_B^2/\alpha_0$ to get the $g$-factor,

$$g_\perp^c \approx \frac{l_B^2}{\alpha_0}\left(E_{0+} - E_{0-}\right) \tag{D10}$$

$$= g_\perp^p + \frac{1}{\sqrt{-\gamma_\parallel^p}}\left(\frac{\beta_1^p l_x}{\alpha_0}\right)^2 . \tag{D11}$$

### Appendix E: Consistency of the theory for wide channels

The behavior of $g_\perp^c$ and $\beta_1^c$ is inconsistent with the principle that the quantum well values should be recovered as $l_x \to \infty$. Fig. 2c and 2d of the main Article show that $g_\perp^c$ and $\beta_1^c$ tend to zero if $l_x \gg \alpha_0 \left| g_\perp^p / [(\gamma_\parallel^p)^{1/4} \beta_1^p] \right|$, and that only if $\beta_1^p = 0$ does $g_\perp^c$ tends to its respective quantum well value. In this section, we show that the theory employed for the quantum channel *is* in fact coherent, despite what Fig. 2 might suggest.

Here we demonstrate that the energy dispersion of the channel orbitals versus $B$ converge to the fan-diagram of the QW system as $l_x \to \infty$. We select the following heterostructure parameters: $l_z = 15\,\text{nm}$, $x = 16\%$, and $F_z = 6\,\text{V}/\mu\text{m}$, such that $\beta_1^p \neq 0$. The fan-diagram of the QW ground state is computed with the method outlined at the end of Section A above, and is shown in Fig. 2 (bottom right). In contrast to HH levels, where the fan-diagram opens up linearly with $B$, a LH fan-diagram opens as $\sqrt{B}$ near $B = 0$ if $\beta_1^p \neq 0$.

This fan-diagram is shown alongside the dispersions obtained from (A12) for finite $l_x$. As $l_x$ increases, the energy gap between adjacent QC orbitals decreases as expected. Coupling between orbitals cause the $g$-factor of the lowest QC orbital to become very small: this is noticeable already from $l_x \geq 58\,\text{nm}$ (see Fig. 2 below, first panel), as the Zeeman energy splitting for the $N = 0$ orbital is much smaller than that of $N \geq 1$ orbitals. For very large $l_x$, orbitals gather closely near $B = 0$, but remain well separated at larger fields. As $l_x \to \infty$, the orbitals spectacularly reorder themselves such that the fan-diagram of the last panel is roughly recovered. The level reordering implies that beyond some value of $l_x$, $g_\perp^c$ does not represent the $g$-factor of the QW ground state anymore.

The energy level structure computed from (A12) does not show all spin-split pairs like the fan-diagram does. This is merely an artifact of the eigenvalue sorting method. In the former, all levels closest to a given energy guess are shown, whereas in the former, all *Landau* levels closest to an energy guess are shown.

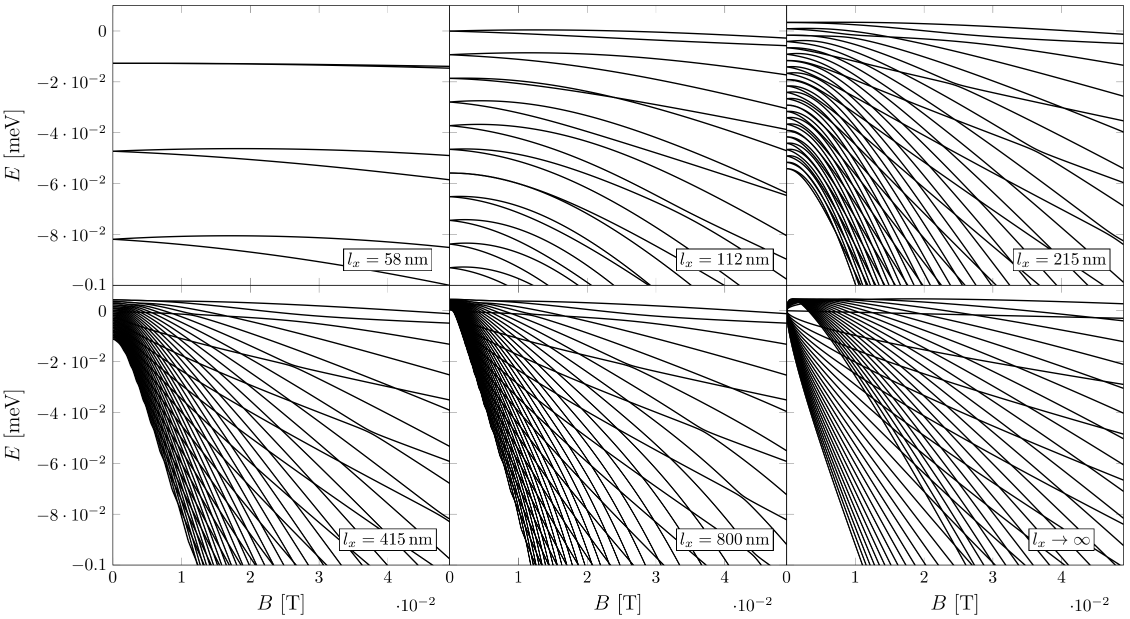


FIG. 2. Quantum channel energy dispersion as a function of the out-of-plane magnetic field up to 0.05 T for increasing widths $l_x$. The bottom right panel labeled $l_x \to \infty$ is the fan-diagram of the QW system. All other panels are computed from (A12) with $k_y = 0$. QW parameters in all cases are $l_z = 15\,\mathrm{nm}$, $x = 16\%$ and $F_z = 6\,\mathrm{V/\mu m}$ ($\beta_1^p \approx 1.21\,\mathrm{meV\,nm}$). The zero of energy is placed on the QW L1 subband ($E_1^{\mathrm{L}} = 0$).

### Appendix F: $\mathrm{Ge}_{1-x}\mathrm{Sn}_x$ Material parametrization

Most of the material parameters of bulk $\mathrm{Ge}_{1-x}\mathrm{Sn}_x$ (with the exception of the three Luttinger parameters $\gamma_{1,2,3}$) are calculated on the full composition range $x \in [0, 1]$ according to a Vegard relation between the parameters of pure Ge and pure Sn. For instance, the parameter $P(x)$ is given by

$$P(x) = (1 - x)P^{\mathrm{Ge}} + xP^{\mathrm{Sn}} - x(1 - x)b_P, \tag{F1}$$

where $P^{\mathrm{Ge}}$ and $P^{\mathrm{Sn}}$ refer to the parameter of pure Ge and pure Sn, respectively, and $b_P$ is a bowing for parameter $P$, if available.

The three Luttinger parameters $\gamma_{1,2,3}$ are interpolated within the composition range $x \in [0, 0.2]$ by fitting a Vegard relation on the parameters reported in Reference 4. The Luttinger parameters are therefore given by

$$\gamma_i(x) = \left(1 - \frac{x}{0.2}\right)\gamma_i^{\mathrm{Ge}} + \frac{x}{0.2}\gamma_i^{(0.2)} - \frac{x}{0.2}\left(1 - \frac{x}{0.2}\right)b_{\gamma_i}, \tag{F2}$$

where $\gamma_1^{(0.2)} = 29.2108$, $\gamma_2^{(0.2)} = 12.2413$ and $\gamma_3^{(0.2)} = 13.7387$ are the values at $x = 0.2$. The bowing parameters are $b_{\gamma_1} = 20.3391$, $b_{\gamma_2} = 9.6609$ and $b_{\gamma_3} = 9.8187$. All other parameters used in the $k \cdot p$ framework are shown in Table I.

TABLE I. Material parameters and bowings of the 6-band $k \cdot p$ framework.

| | | Ge | $Ge_{1-x}Sn_x$ | Sn |
|---|---|---|---|---|
| Lattice constant | | | | |
| $a_0$ | [Å] | $5.652357^{a}$ | $-0.083^{g}$ | $6.480117^{b}$ |
| Bulk band energies | | | | |
| $\mathcal{E}_{\Gamma_5^+}$ | [eV] | 0 | | $0.69^{h*}$ |
| $\Delta_0$ | [eV] | $0.290^{b}$ | $-0.100^{g}$ | $0.770^{f}$ |
| Elastic constants | | | | |
| $c_{12}/c_{11}$ | | $0.333^{b}$ | | $0.425^{b}$ |
| Deformation potentials | | | | |
| $a_v$ | [eV] | $1.24^{c}$ | | $1.58^{i}$ |
| $b$ | [eV] | $-2.86^{d}$ | | $-2.7^{j}$ |
| Effective mass and spin parameters | | | | |
| $\gamma_1$ | | $13.38^{e}$ | † | † |
| $\gamma_2$ | | $4.24^{e}$ | † | † |
| $\gamma_3$ | | $5.69^{e}$ | † | † |
| $\kappa$ | | $3.41^{f}$ | | $-11.84^{f}$ |
| $q$ | | $0.06^{e}$ | | $0.30^{f}$ |

References: [a]:[5], [b]:[6], [c]:[7], [d]:[8], [e]:[9], [f]:[10], [g]:[11], [h]:[12], [i]:[13], [j]:[14]

* Relative to Ge

† See (F2)


[1] P. Del Vecchio and O. Moutanabbir, Phys. Rev. B **107**, L161406 (2023).

[2] P. Del Vecchio and O. Moutanabbir, Phys. Rev. B **110**, 045409 (2024).

[3] J. M. Luttinger, Phys. Rev. **102**, 1030 (1956).

[4] K. Lu Low, Y. Yang, G. Han, W. Fan, and Y.-C. Yeo, Journal of Applied Physics **112**, 103715 (2012).

[5] R. R. Reeber and K. Wang, Materials Chemistry and Physics **46**, 259 (1996).

[6] O. Madelung, ed., *Semiconductors, Group IV Elements and III-V Compounds* (Springer-Verlag Berlin Heidelberg, 1991).

[7] C. G. Van de Walle, Phys. Rev. B **39**, 1871 (1989).

[8] C. G. Van de Walle and R. M. Martin, Phys. Rev. B **34**, 5621 (1986).

[9] R. Winkler, *Spin-orbit Coupling Effects in Two-Dimensional Electron and Hole Systems*, Vol. 191 (Springer, 2003).

[10] P. Lawaetz, Phys. Rev. B **4**, 3460 (1971).

[11] M. P. Polak, P. Scharoch, and R. Kudrawiec, Journal of Physics D: Applied Physics **50**, 195103 (2017).

[12] J. Menéndez and J. Kouvetakis, Applied Physics Letters **85**, 1175 (2004).

[13] T. Brudevoll, D. S. Citrin, M. Cardona, and N. E. Christensen, Phys. Rev. B **48**, 8629 (1993).

[14] M. Willatzen, L. C. Lew Yan Voon, P. V. Santos, M. Cardona, D. Munzar, and N. E. Christensen, Phys. Rev. B **52**, 5070 (1995).
